# Supplementary material for: Is Reinforcement Learning (Not) for Natural Language Processing: Benchmarks, Baselines, and Building Blocks for Natural Language Policy Optimization
Source: arXiv:2210.01241 source file (2023-03-01)
Supplement: Supplementary file 1 [file ppo.tex]

\subsubsection{PPO All-in-One}
\kb{Borrowed from: https://spinningup.openai.com/en/latest/algorithms/ppo.html }
\begin{algorithm}[h]
    \caption{PPO}
    \begin{algorithmic}
      \STATE {\bfseries Input:} initial policy parameters $\theta_0$
      \STATE {\bfseries Input:} initial value function parameters $\phi_0$
      \REPEAT
          \STATE Collect set of trajectories $\mathcal{D}_m = \{  \tau_i\}$ by running policy $\pi_{\theta_m}$ in the environment.
          \STATE Compute rewards-to-go $\hat{R}_t$
          \STATE Compute the advantage estimate $\hat{A}_t$
          \STATE Update the policy by maximizing the PPO-Clip objective:\\
          $$\theta_{m+1} = \text{argmax}_{\theta} \frac{1}{\vert \mathcal{D}_m\vert T } \sum_{\tau \in \mathcal{D}} \sum_{\tau=0}^{T} \min \Big( \frac{\pi_{\theta}(a_t \vert s_t)}{\pi_{\theta_m}(a_t \vert s_t)} A^{\pi_{\theta_m}}, g(\epsilon, A^{\pi_{\theta_m}}(s_t, a_t)) \Big)$$\\
          \STATE Fit value function by regression on mean-squared error:\\
          $$\phi_{m+1}= \text{argmin}_\phi \frac{1}{\vert \mathcal{D}_m \vert T} \sum_{\tau \in \mathcal{D}_m} \sum_{t=0}^{T} \Big( V_\phi(s_t) - \hat{R}_t \Big)^2$$\\
      \UNTIL{convergence}
    \end{algorithmic}
  \end{algorithm}

\clearpage
\subsubsection{Ablation Study}
Below are list of things to studied:
\begin{itemize}
    \item Effect of decoding during rollouts and how it affects exploration and stability
        \subitem(https://arxiv.org/pdf/2202.11818.pdf)
    \item  Consistent Dropout for Policy Gradient Reinforcement Learning 
    \item  NLPO hyperparams (top p, target update frequency)
    \item  Reward hacking on PPO (vs NLPO)  - with and without penalty term
    
\end{itemize}

\subsubsection{Hyperparameters}
